# Supplementary material for: Machine-learning effective many-body potentials for anisotropic particles using orientation-dependent symmetry functions
Source: arXiv:2207.06065 source file (2022-07-13)
Supplement: Supplementary file 1 [file SM_SFS-Rods.pdf]

# Machine-learning effective many-body potentials for anisotropic particles using orientation-dependent symmetry functions

Gerardo Campos-Villalobos,<sup>\*</sup> Giuliana Giunta, Susana Marín-Aguilar, and Marjolein Dijkstra<sup>†</sup>*Soft Condensed Matter, Debye Institute for Nanomaterials Science, Department of Physics, Utrecht University, Princetonplein 1, 3584 CC Utrecht, The Netherlands*

## I. SYMMETRY FUNCTION PARAMETERS

Parameters used to construct the initial pool of candidate symmetry functions for building the effective potentials for the different models are reported in Table I. The optimal subset of symmetry functions (SFs) for each case is selected according to the feature selection scheme described in the main text. A single cut-off value is used in each case to construct the effective potentials. In particular, we choose  $r_c/\sigma_0 = 6.5$ ,  $r_c/\sigma_c = 7.0$ ,  $r_c/\sigma_A = 6.5$  and  $r_c/D = 8.0$  for the Gay-Berne ellipsoids, colloid-polymer mixtures, core-shell microgel rods and ligand-stabilized nanorods, respectively.

TABLE I Parameters used to generate the initial pool of candidate SFs. System I: Gay-Berne ellipsoids; System II: Colloid-polymer mixture; System III: Core-shell microgel rods; System IV: Ligand-stabilized nanorods. Units are shown in brackets.

| SF                        |                  | I                                                          | II                                                         | III                                                        | IV                                                  |
|---------------------------|------------------|------------------------------------------------------------|------------------------------------------------------------|------------------------------------------------------------|-----------------------------------------------------|
| $G^{(2),R}$               | $\eta$           | 0.001,0.01,0.1,<br>1.0,2.0,4.0,8.0 [ $\sigma_0^{-2}$ ]     | 0.001,0.01,0.1,<br>1.0,2.0,4.0,8.0 [ $\sigma_c^{-2}$ ]     | 0.001,0.01,0.1,<br>1.0,2.0,4.0,8.0 [ $\sigma_A^{-2}$ ]     | 0.001,0.01,0.1,1.0,2.0<br>[ $D^{-2}$ ]              |
|                           | $R_s$            | 0.0,0.1,0.2,0.3,0.4,<br>0.5,0.6,0.7,0.8,0.9 [ $\sigma_0$ ] | 0.0,0.1,0.2,0.3,0.4,<br>0.5,0.6,0.7,0.8,0.9 [ $\sigma_c$ ] | 0.0,0.1,0.2,0.3,0.4,<br>0.5,0.6,0.7,0.8,0.9 [ $\sigma_A$ ] | 0.0,0.1,0.2,0.3,0.4<br>[ $D$ ]                      |
| $G^{(2),OD_1}/G^{(3),OD}$ | $\sigma_{  }$    | 0.8,0.9,1.0,1.6,1.7,<br>1.8,1.9,2.0,2.1,2.2 [ $\sigma_0$ ] | 3.1,3.2,3.3,3.4,3.5<br>[ $\sigma_c$ ]                      | 3.1,3.2,3.3,3.4,3.5<br>[ $\sigma_A$ ]                      | 3.2,3.3,3.5,3.6,3.7,3.8<br>[ $D$ ]                  |
|                           | $\sigma_{\perp}$ | 0.40,0.55,0.60,0.65,<br>0.70,0.75,0.80 [ $\sigma_0$ ]      | 0.55,0.60,0.65,0.70,0.75<br>[ $\sigma_c$ ]                 | 0.55,0.60,0.65,0.70,0.75<br>[ $\sigma_A$ ]                 | 0.7,0.8,0.9,1.0,1.1<br>[ $D$ ]                      |
| $G^{(2),OD_2}$            | $\alpha$         | -                                                          | 0.001,0.01,0.1,<br>1.0,2.0,4.0,8.0 [ $\sigma_c^{-2}$ ]     | 0.001,0.01,0.1,<br>1.0,2.0,4.0,8.0 [ $\sigma_A^{-2}$ ]     | 0.001,0.01,0.1,<br>1.0,2.0,4.0,8.0 [ $D^{-2}$ ]     |
|                           | $R_m$            | -                                                          | 0.0,0.1,0.2,0.3,0.4,<br>0.5,0.6,0.7,0.8,0.9 [ $\sigma_c$ ] | 0.0,0.1,0.2,0.3,0.4,<br>0.5,0.6,0.7,0.8,0.9 [ $\sigma_A$ ] | 0.0,0.1,0.2,0.3,0.4,<br>0.5,0.6,0.7,0.8,0.9 [ $D$ ] |
| $G^{(3),OD}$              | $\lambda$        | -                                                          | -1,1                                                       | -1,1                                                       | -                                                   |
|                           | $\xi$            | -                                                          | 1,2,4,8                                                    | 1,2,4,8                                                    | -                                                   |

<sup>\*</sup>Electronic address: [g.d.j.camposvillalobos@uu.nl](mailto:g.d.j.camposvillalobos@uu.nl)

<sup>†</sup>Electronic address: [m.dijkstra@uu.nl](mailto:m.dijkstra@uu.nl)

## II. LEARNING CURVES

In Fig. 1a we show the root mean square errors (RMSE) of the linear fits with the actual potential of mean force of a pair of ligand-stabilized nanorods as a function of the number of selected SFs for both the training and the test sets. Fig. 1b shows the type of descriptor that is sequentially selected from the pool of candidate SFs according to the feature selection scheme discussed in the main text.

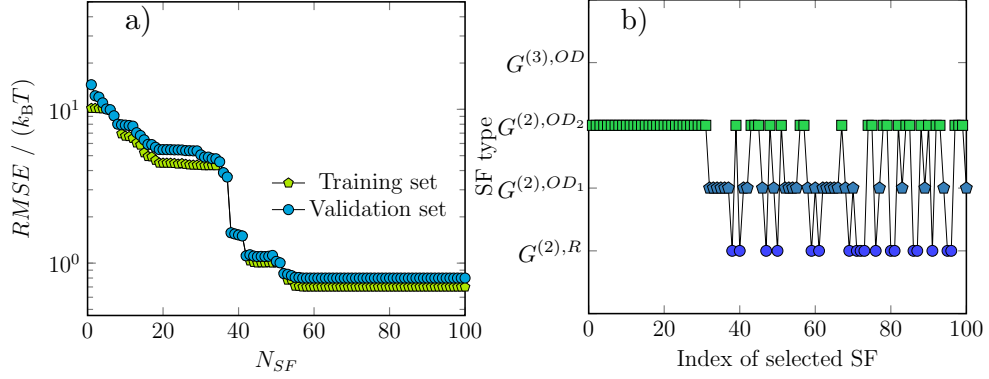

FIG. 1 a) Root mean square error (RMSE) as a function of the number of SFs in the subset  $N_{SF}$  for the ligand-stabilized nanorods. The RMSE values are shown for the training and validation sets. b) Type of SF as a function of the index chosen in the feature selection method.

Learning curves showing the accuracy of the constructed models on the validation and training examples as a function of the number of training examples are shown in Figs. 2, 3, 4 and 5 for the Gay-Berne dimers and trimers, one-component effective Hamiltonian of colloid-polymer mixtures, core-shell microgel rods and ligand-stabilized nanorods, respectively. The procedure to extract the learning curves is as follows: first, for each data set, a 80/20 training/validation split is performed. Secondly, various subsets with diverse numbers of examples taken randomly from the whole training datasets are constructed. Finally, for each subset of examples, a feature selection and subsequent linear regression is performed as described in the main text. The RMSE reported in the learning curves are those computed with the linear fits using  $N_{SF} = 70, 120, 50$  and  $50$  descriptors for the Gay-Berne dimers and trimers, one-component effective Hamiltonian of colloid-polymer mixtures, core-shell microgel rods and ligand-stabilized nanorods, respectively. We note that in all cases, the number of examples used for training enables the construction of predictive models that generalize accurately to configurations reserved in the validation sets.

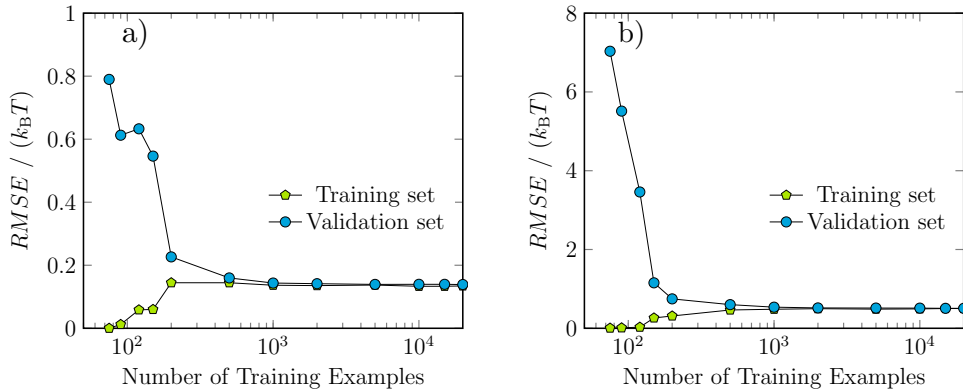

FIG. 2 Learning curves showing the model accuracy (RMSE) on training and validation examples as a function of the number of training examples. Results are shown for the models of dimers (a) and trimers (b) of Gay-Berne ellipsoidal particles constructed with  $N_{SF} = 70$   $G^{(2),OD_1}$  descriptors.

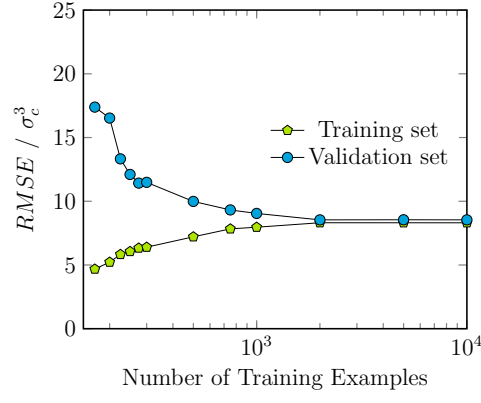

FIG. 3 Learning curve showing the accuracy (RMSE) of the model for colloidal hard rods and nonadsorbing polymer on training and validation examples as a function of the number of training examples.

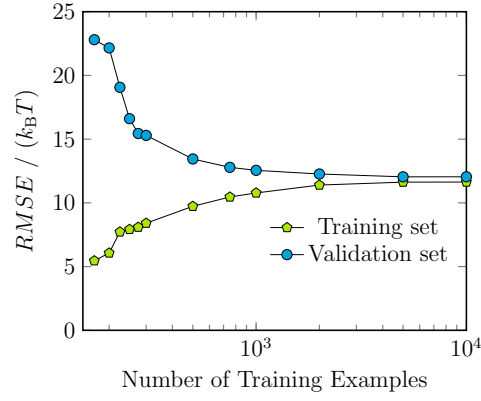

FIG. 4 Learning curve showing the accuracy (RMSE) of the model for core-shell microgel rods on training and validation examples as a function of the number of training examples.

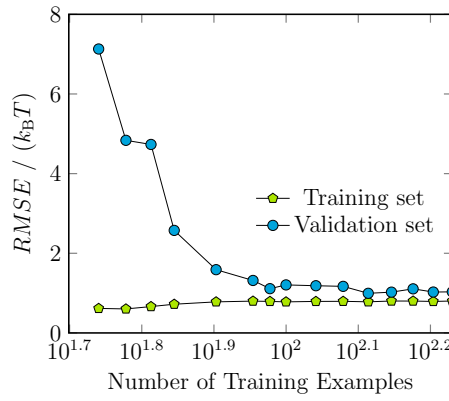

FIG. 5 Learning curve showing the accuracy (RMSE) of the model for ligand-stabilized nanorods on training and validation examples as a function of the number of training examples.

### III. COMPUTATIONAL EFFICIENCY OF THE POTENTIALS

Here, we briefly discuss the computational cost of evaluating the ML potentials. We start by extracting the computational time required for the evaluation of the effective ML potentials ( $\tau_{\text{ML}}$ ) on trimers of Gay-berne ellipsoidal particles. In particular, we select 250 configurations from the trimers contained in our training data set and evaluate the serial computing times for the calculation of the total energy. We repeat the evaluation of the energy on each configuration 500 times to get the average of  $\tau_{\text{ML}}$ . To better appreciate the difference between the cost associated to each type of descriptor, we evaluate the ML potentials constructed as linear combinations of a number  $N_{SF}$  of SFs of the same type. The resulting values are shown in Fig. 6. As expected, the spherically-symmetric  $G^{(2),R}$  SFs are those with the lowest computational times as they only depend on the center-of-mass distance between pairs of particles. In contrast, the orientation-dependent SFs (ODSFs) ( $G^{(2),OD_1}$ ,  $G^{(2),OD_2}$  and  $G^{(3),OD}$ ) imply a higher cost as they also depend on the orientation of the particles. In particular, the ML potentials constructed solely with the three-body ODSFs ( $G^{(3),OD}$ ) are naturally the most expensive ones as they additionally depend on the angle between triplets of particles.

As discussed in the main text, the functional form of the ML potentials for the non-spherical particles is  $\Phi(\{\mathbf{R}_i, \hat{\mathbf{u}}_i\}) = \sum_i^N \sum_l^{N_{SF}} \omega_l G_l(i)(\{\mathbf{R}_i, \hat{\mathbf{u}}_i\})$ , where  $i$  runs over all particles and  $l$  runs over the descriptor ( $G_l(i)$ ) describing the local environment of particle  $i$ ,  $\omega_l$  are the coefficients (weights) fixed by the fitting procedure. Therefore, this implies that, if we use no tricks, the computational cost of evaluating the total energy in a system of  $N$  particles using a ML potential based on two- and three-body SFs could be expected to scale as  $N^2 N_{SF}$  and  $N^3 N_{SF}$ , respectively. This justifies the feature selection procedure in our approach because controlling the number  $N_{SF}$  of descriptors directly influences the computational cost of the resulting potentials.

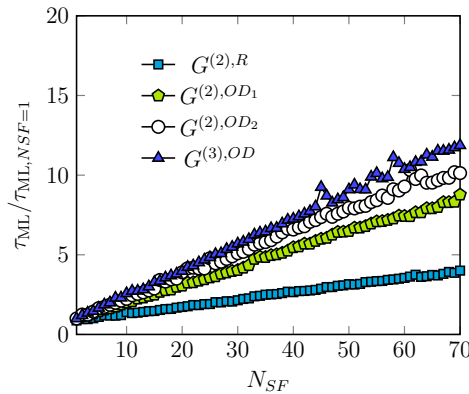

FIG. 6 Computational time required for the evaluation of the total energy in a system of three ellipsoidal particles using a ML potential ( $\tau_{\text{ML}}$ ) constructed with a number of descriptors  $N_{SF}$  of different type as labelled. All values are divided by  $\tau_{\text{ML}}$  of a single SF.

To compare the computational cost of our ML potential for ellipsoids (constructed with  $N_{SF} = 70$   $G^{(2),OD_1}$  ODSFs) with that of the “true” system, we also extract the CPU time for the evaluation of the total energy of the trimer configurations using the Gay-Berne pair potential  $\tau_N$  (see Sec. IIIA of the main text). The average ratio measured over 250 configurations and repeated 500 times is  $\tau_N / \tau_{\text{ML}} \approx 5 \times 10^{-2}$ , indicating that the cost of the ML potential for this specific case is about 20 times larger than that of the original model. This dramatic slowdown is clearly expected for this system due to the simple functional form of the Gay-Berne pair potential. As we state in the main text, such a system was presented as an example to illustrate the suitability of our proposed ODSFs to describe the local environment of prolate ellipsoidal particles and to construct accurate ML potentials. The approach we present is intended to be applied to construct (many-body) effective potentials of non-spherical particles with underlying or fine-grained complex interactions. In fact, for the cases of colloid-polymer mixtures and core-shell microgel rods we observe a significant speedup. The ratios  $\tau_N / \tau_{\text{ML}}$  are extracted by selecting 10 decorrelated configurations for each colloid packing fraction ( $\eta_c$ ) from the training data set, evaluating the serial computing times for the calculation of the many-body effective potentials and repeating this procedure 20 times to get the average ratios. In the numerical evaluation of the many-body potential of the colloid-polymer mixture we use a spherocylindrical grid of points to evaluate the free volume by integration (Campos-Villalobos *et al.*, 2021). This consists of a combination of a spherically-symmetric ( $r^3, \cos(\theta), \phi$ ) grid of 100, 50 and 25 points, respectively (for the semi-spherical caps) and a cylindrical grid with 100, 50 and 250 points in  $(r, \theta, z)$ , respectively. For the core-shell microgel rods, the deformable surface of each of the 5 spheres is discretized into 200 points. The measured  $\tau_N / \tau_{\text{ML}}$  values as a function of  $\eta_c$ , for the two different systems, are reported in Fig. 7. We find that our ML potentials speed up the many-body potential evaluation at least by three

orders of magnitude for the colloid-polymer mixture. In the case of the microgel rods, the speedup is less marked, but still significant as the ratio is  $\tau_N/\tau_{ML} \approx 3$ .

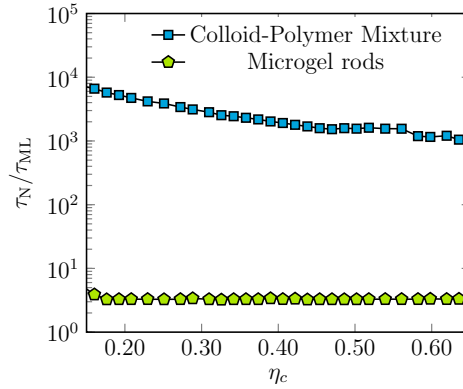

FIG. 7 Ratio between the computational time required for the numerical evaluation of the many-body term ( $\tau_N$ ) and the ML potential ( $\tau_{ML}$ ) as a function of colloid packing fraction  $\eta_c$  of a colloid-polymer mixture (blue squares) and of core-shell microgel rods (green pentagons).

The observed speedup achieved with our ML potentials can be rationalized by considering the order of the computations on which they are based. When the many-body potential of the fine-grained model is evaluated numerically (using a grid of  $\mathcal{M}$  points) in a system of  $N$  colloidal anisotropic particles, the computational time scales as  $N^2\mathcal{M}$ . In contrast, by assuming that the computational cost of the ML potential is dominated by the most expensive three-body ODSFs, the time required for the evaluation scales as  $N^3N_{SF}$ . Thus, as a rough guideline, one can expect a significant speedup if the condition  $\mathcal{M}/N > N_{SF}$  is satisfied. In practice, this strongly depends on the type of interactions in the fine-grained model (how the potential is determined by the  $\mathcal{M}$  points), on model parameters (e.g. cut-off values used for the construction of the ML potentials) and on the final algorithmic implementation. In the case of ML potentials built with two-body descriptors, the condition for observing a marked speedup would be simply  $\mathcal{M} > N_{SF}$ , which will generally hold valid as we have seen that using the feature selection method described in the main text, allows the construction of high-accuracy models with a relatively small number of descriptors  $N_{SF}$ . In the case of the fine-grained model of ligand-stabilized nanorods (Sec. III D of the main text), the total interaction is determined by non-bonded (pair) and bonded (bond stretching and angle bending) potentials. For each nanorod, a total of 10566 sites (CG beads) representing the core atoms and ligand chains are used. Thus the simple scaling mentioned above would point already to a significant speedup of the simulations using the ML potential. In addition to this, it is important to consider that the “learned” effective two-body interaction (potential of mean force) between pairs of nanorods is extracted by integrating out the degrees of freedom of the ligands. This potential of mean force is the CG potential, whose force is exactly the mean force over all corresponding fine-grained structures. Such a “bottom-up” coarse-graining is based on a mapping that effectively projects fine-grained states onto a lower-dimensional representation, which allows to access larger time- and length-scales. Therefore, determining a more precise computational gain of the CG ML potentials relative to that of the fine-grained models would require a more extensive exploration based on actual simulations for the calculation of system properties. We note that although here we have only discussed serial computing times, the descriptors can also be evaluated using parallelization.

## References

Campos-Villalobos, G., E. Boattini, L. Filion, and M. Dijkstra, 2021, J. Chem. Phys. **155**(17), 174902.
